# Supplementary material for: EMMA: A New Platform to Evaluate Hardware-based Mobile Malware Analyses
Source: arXiv:1603.03086 source file (2016-03-11)
Supplement: Supplementary file 1 [file results-appendix.tex]

\section{Additional Results}

%%%%%%%%%%%%%
\subsection{Sensitivity to Machine Learning Parameters}

%-------------------
\begin{figure}[tbp]
   \centering
   \includegraphics[width=0.45\textwidth]{figs/PLOTS_FINAL/3.parameter-variation/phase_level_200_traces.pdf}\par
   \caption{Performance v. machine learning parameters. Figure shows a small representative subset of 200 parameter combinations.}
   \label{fig:param-var-200}
\end{figure}
%-------------------

%-------------------
\begin{figure}[tbp]
   \centering
   \includegraphics[width=0.45\textwidth]{figs/PLOTS_FINAL/3.parameter-variation/phase_tp_vs_phase_fp_PARAM_5.pdf}\par
\caption{Detection accuracy v. warning time parameter (in number of phase windows below detection threshold)}
\label{fig:param-5}
\end{figure}
%-------------------

Before choosing good Markov model parameters for every application, we
searched the parameter space to determine how sensitive the ML model is to
particular parameters. When analyzing results, we observed global and
app-specific trends. In this section, we summarize our findings using
AngryBirds as an example. In these experiments, we varied the basic parameters
such as phase-window size, detection window size, wavelet type and level,
number of distinct execution phases and etc. Phase window sizes together with
execution phase number dramatically affect the model quality.  When we set the
number of execution phases too big, this usually worsens the detection rate
because the number of distinct phases in the application is not very high.

One of the most recent experiments with different parameter settings is
presented on the Fig.~\ref{fig:param-var-200}. The highlighted curve corresponds to the chosen
parameter settings. This curve is not the best possible curve according this
picture, but we chose those parameter settings by maximizing detection rate of
various synthetic malware samples while minimizing the phase-level false
positive rate. In general,
parameter settings, which provide the best detection rate in terms of
individual synthetic payloads, do not ensure the best detection rate in terms
of phase windows.

The next interesting parameter we would like to point out is the number of
consecutive phases that are considered when the model decides whether to raise
an alarm or not. We varied this parameter from 1 up to 50 (Fig.~\ref{fig:param-5}). The
observation we can make regarding the value of this parameter is that the lower
parameter is, the more malicious phase-level windows we can detect, however,
the price of this is the hfGigh level of false positives. If we increase this
parameter, the detection rate quickly reaches its saturation point and its
upper bound is significantly less than the upper bound of the detection rates
corresponding to the lower values of the parameter (curve 1 and curve 50).
Experimenting with different values of this parameter shows that the value 5,
which we chose for all experiments, provides acceptable results.

\ignore{
Throughout the paper we measure detection rate in terms of individual phase
windows. Counting false positives and true positives over individual
phase-level windows is useful for precise estimation of accuracy of the ML
pipeline, but is not very practical. We also analyzed how the number false
positives changes if we increase time window  size, which we classify as
malicious or benign, from five phase-level windows up to the length of a trace
(fig. \ref{fig:param-time-window}). The low bound is equal to five  phase-level windows because our
implementation of a Markov model needs to observe the current phase-level
window and the four  previous windows to classify the current window. False
positive rate depends also on the threshold value used in the Markov model,
that is why we repeated the experiment for three different values of the
threshold. The larger the size of the time window is, the higher the false
positive rate is. This result is expectable: if we use very large time-window,
than with high probability there exist five consecutive points below the
threshold.  The lower threshold is, the longer we can stay in the region with
reasonable number of false positives while varying the time-window size, but
eventually we hit 100\% false positive level for very large time-windows. This
experiment shows that the definition of detection rate in terms of
(mis)classified windows is not invariant - it depends on the length of the time
windows.
}
%%%%%%%%%%%%%
\subsection{Synthetic Malware on Sana App}

%-------------------
\begin{figure*}[tbp]
\begin{minipage}[tbp]{0.33\linewidth}
   \includegraphics[width=\textwidth]{figs/PLOTS_FINAL/6.b.Sana-examples/25.pdf}\par
   \label{fig:ab-1}
\end{minipage}
%\hfill
\begin{minipage}[tbp]{0.33\linewidth}
   \includegraphics[width=\textwidth]{figs/PLOTS_FINAL/6.b.Sana-examples/26.pdf}\par
   \label{fig:ab-2}
\end{minipage}
\begin{minipage}[tbp]{0.33\linewidth}
   \includegraphics[width=\textwidth]{figs/PLOTS_FINAL/6.b.Sana-examples/28.pdf}\par
   \label{fig:ab-3}
\end{minipage}
\caption{Sana medical app with increasing number of SMSs stolen.}
\label{fig:sana-sms}
\end{figure*}
%-------------------

Figure~\ref{fig:sana-sms} shows how Sana medical app's signature is affected by 
the insertion of an SMS stealer, with increasing number of SMSs being stolen.
As SMSs theft increases, the probability curve goes lower and stays low longer, 
thus indicating anomalous behavior compared to the baseline Sana application.

\subsection{Performance counters}

The performance counters used in our study are listed in Figure~\ref{fig:perf_counters_choice}.

\begin{figure}[tbp]
\centering
\includegraphics[width=0.35\textwidth]{figs/perf-counters.pdf}\par
\caption{Choice of performance counters}
\label{fig:perf_counters_choice}
\end{figure}
